# Supplementary material for: The Impact of Hyperparameters on Large Language Model Inference Performance: An Evaluation of vLLM and HuggingFace Pipelines
Source: arXiv:2408.01050 source file (2024-08-02)
Supplement: Supplementary file 1 [file appendix.tex]

\section{Appendix}

\subsection{Description of dataset HumanEval SingleLine}

\begin{table*}[t]
\centering
\begin{tabular}{|l|rr|rr|rr|rr|rr|rr|}
\toprule

model & gpus & tp & gpus & e/t & gpus & en ef & gpus & \% GPU &gpus & \% Mem & gpus & \% CPU \\
\midrule
bloom-1b7 & 1 & 133.1 & 1 & 3.8 & 1 & 35.119 & 1 & 27.2 & 2 & 82.3 & 8 & 3.4 \\
bloom-3b & 1 & 98.6 & 1 & 5 & 1 & 19.566 & 1 & 35.1 & 4 & 83.1 & 8 & 3.9 \\
bloom-7b1 & 2 & 67.2 & 1 & 7.8 & 1 & 8.174 & 1 & 50.7 & 2 & 83.2 & 8 & 4 \\
CodeLlama-13b-hf & 4 & 48.2 & 1 & 7.6 & 1 & 4.679 & 1 & 81 & 8 & 87 & 8 & 2 \\
CodeLlama-34b-hf & 8 & 34.7 & 4 & 32.3 & 4 & 1.002 & 4 & 56.3 & 8 & 85.3 & 8 & 2.3 \\
CodeLlama-70b-hf & 8 & 21.7 & 8 & 76.9 & 8 & 0.282 & 8 & 61.7 & 8 & 85.4 & 8 & 2.6 \\
CodeLlama-7b-hf & 1 & 63 & 1 & 4.4 & 1 & 14.193 & 1 & 70.5 & 8 & 87.2 & 8 & 2 \\
Codestral-22B-v0.1 & 8 & 64.7 & 2 & 17.4 & 4 & 2.469 & 2 & 62.1 & 8 & 83.2 & 8 & 1.9 \\
gemma-2b & 1 & 132.3 & 1 & 2.1 & 1 & 61.701 & 1 & 54.8 & 1 & 81.7 & 8 & 1.8 \\
gemma-7b & 4 & 70.8 & 1 & 6.5 & 1 & 7.811 & 1 & 57.3 & 4 & 82.1 & 8 & 1.9 \\
Mistral-7B-v0.1 & 4 & 66.5 & 1 & 4.5 & 1 & 13.983 & 1 & 71.8 & 4 & 83.4 & 8 & 1.9 \\
Mixtral-8x7B-v0.1 & 4 & 59.2 & 4 & 19.6 & 4 & 3.021 & 4 & 45.6 & 4 & 82.8 & 8 & 2 \\
phi-1 & 1 & 158.5 & 1 & 1.8 & 1 & 89.227 & 1 & 26.4 & 2 & 86.5 & 8 & 1.8 \\
phi-1\_5 & 1 & 171.5 & 1 & 1.6 & 1 & 107.498 & 1 & 43.1 & 4 & 86.5 & 8 & 1.8 \\
phi-2 & 1 & 110.3 & 1 & 2.9 & 1 & 37.483 & 1 & 36.2 & 2 & 87.5 & 8 & 1.9 \\
starcoder & 8 & 58.4 & 1 & 8.4 & 1 & 3.856 & 1 & 82.7 & 4 & 86.9 & 8 & 2.1 \\
starcoder2-3b & 1 & 104.1 & 1 & 2.7 & 1 & 38.672 & 1 & 55.1 & 4 & 86.4 & 8 & 1.9 \\
starcoder2-7b & 4 & 62.3 & 1 & 4.7 & 1 & 12.958 & 1 & 71 & 4 & 86.3 & 2 & 1.5 \\
WizardCoder-15B-V1 & 8 & 57.3 & 1 & 10.5 & 2 & 3.27 & 1 & 66.6 & 2 & 86.7 & 8 & 2 \\
WizardCoder-33B-V1.1 & 8 & 43.8 & 4 & 30.1 & 4 & 1.221 & 4 & 60.1 & 8 & 77.4 & 8 & 2 \\
\bottomrule
\end{tabular}
\caption{ vLLM}
\label{tab:minMaxMetricAutoHFOnlineInferece}
\end{table*}
